# Supplementary material for: Optical and electronic properties of low-density InAs/InP quantum dot-like structures devoted to single-photon emitters at telecom wavelengths
Source: arXiv:1912.07490 ancillary file (2019-12-16)
Supplement: Supplementary file 1 [file Supplementary.pdf]

# Supplementary information on Optical and electronic properties of low-density InAs/InP quantum dot-like structures devoted to single-photon emitters at telecom wavelengths

P. Holewa,[1] M. Gawełczyk,[2,1] C. Ciostek,[1] P. Wyborski,[1] S. Kadkhodazadeh,[3] E. Semenova,[4] and M. Syperek[1]

[1]*Laboratory for Optical Spectroscopy of Nanostructures, Department of Experimental Physics, Faculty of Fundamental Problems of Technology, Wrocław University of Science and Technology, Wybrzeże Wyspiańskiego 27, 50-370 Wrocław, Poland*

[2]*Department of Theoretical Physics, Faculty of Fundamental Problems of Technology, Wrocław University of Science and Technology, 50-370 Wrocław, Poland*

[3]*DTU Nanolab – National Centre for Nano Fabrication and Characterization, Technical University of Denmark, Kongens Lyngby DK-2800, Denmark*

[4]*DTU Fotonik, Technical University of Denmark, Kongens Lyngby DK-2800, Denmark*

This file is auxiliary information for the manuscript *Optical and electronic properties of low-density InAs/InP quantum dot-like structures devoted to single-photon emitters at telecom wavelengths* by P. Holewa *et al.* This document contains supplementary Figs. 1 and 2, which show high-angle annular dark-field scanning transmission electron microscopy images of surface and buried quantum dots with the wetting layer, as well as Fig. 3 presenting the map of the fractional change in the interplanar lattice spacing.

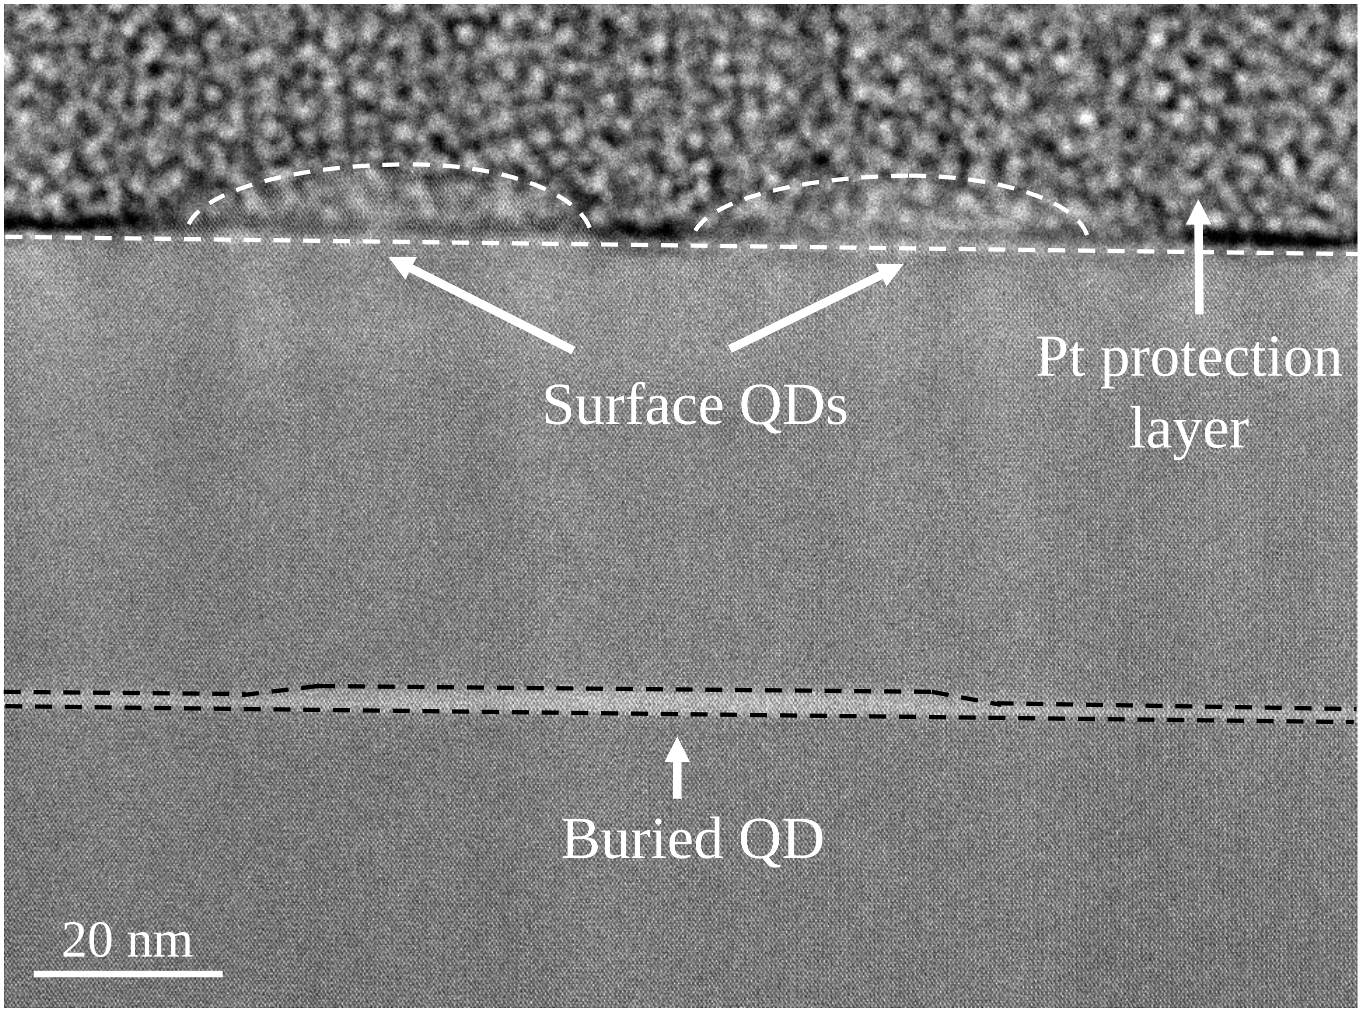


FIG. 1: (a) HAADF STEM image showing a cross-sectional view of the buried and surface QDs along the $[\overline{1}\overline{1}0]$ direction.

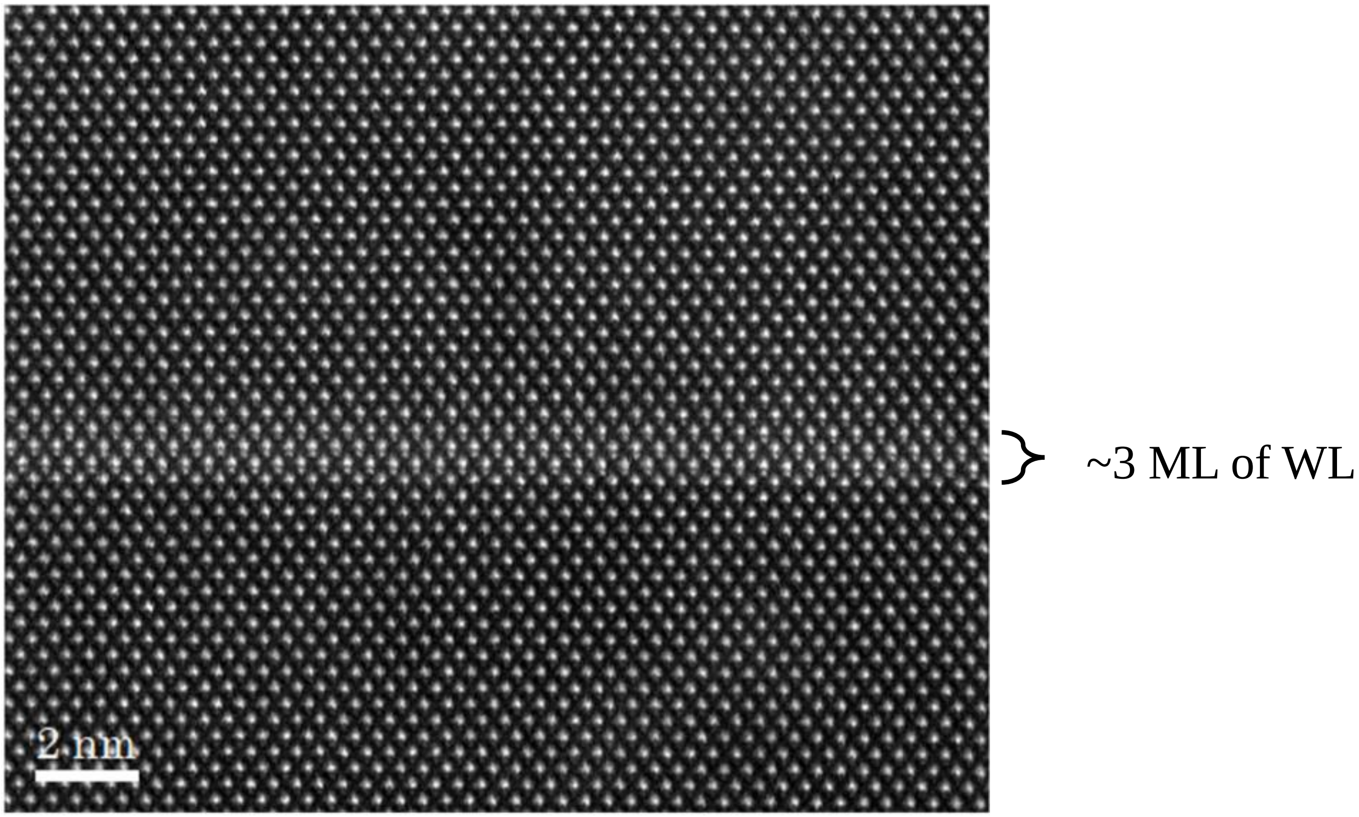


FIG. 2: Atomic resolution HAADF STEM of the WL in the buried QDs viewed along a $[\bar{1}10]$ direction, revealing the WL to be ~3 ML thick.

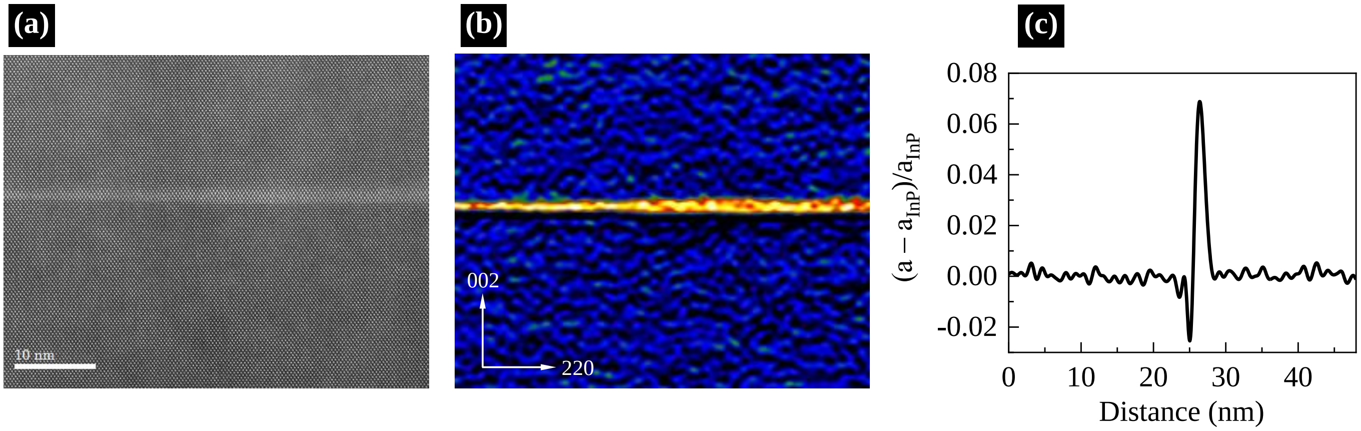


FIG. 3: (a) An atomic resolution HAADF STEM image of a buried QD. (b) The map of the fractional change in the interplanar lattice spacing along the [002] direction $a$ relative to the InP lattice constant $a_{\mathrm{InP}}$: $(a - a_{\mathrm{InP}})/a_{\mathrm{InP}}$, obtained by applying the geometric phase analysis [1] to the image in (a). (c) $(a - a_{\mathrm{InP}})/a_{\mathrm{InP}}$ averaged along the [220] direction, showing values up to 0.07, which converts to ~100 % InAs composition in the buried QD.

[1] M. Hÿtch, E. Snoeck, and R. Kilaas, Quantitative measurement of displacement and strain fields from HREM micrographs, Ultramicroscopy **74**, 131 (1998).
